# Supplementary material for: Tiny Machine Learning: Progress and Futures
Source: arXiv:2403.19076 source file (2024-03-29)
Supplement: Supplementary file 1 [file 6_supp.tex]

\section{Demo Video}
We release a demo video of MCUNet running the visual wake words dataset\cite{chowdhery2019visual} in  \href{https://youtu.be/YvioBgtec4U}{this link}. MCUNet with TinyNAS and TinyEngine achieves \textbf{12\%} higher accuracy and \textbf{2.5$\times$} faster speed compared to MobilenetV1 on TF-Lite Micro~\cite{abadi2016tensorflow}.  

Note that we show the actual frame rate in the demo video, which includes frame capture latency overhead from the camera (around 30ms per frame). Such camera latency slows down the inference from 10 FPS to 7.3 FPS.

\section{Profiled Model Architecture Details}
\label{sup:arch_detail}
We provide the details of the models profiled in Figure~\ref{fig:speedup}.

\myparagraph{SmallCifar.} SmallCifar is a small network for CIFAR~\cite{krizhevsky2009learning} dataset used in the MicroTVM/$\mu$TVM post\footnote{{\url{https://tvm.apache.org/2020/06/04/tinyml-how-tvm-is-taming-tiny}}}. It takes an image of size $32\times32$ as input. The input image is passed through $3\times$ \{convolution (kernel size $5\times5$), max pooling\}. The output channels are 32, 32, 64 respectively. The final feature map is flattened and passed through a linear layer of weight 1024$\times$10 to get the logit. The model is quite small. We mainly use it to compare with MicroTVM since most of ImageNet models run OOM with MicroTVM.

\myparagraph{ImageNet Models.} All other models are for ImageNet~\cite{deng2009imagenet} to reflect a real-life use case. 
The input resolution and model width multiplier are scaled down so that they can run with most of the libraries profiled. We used input resolution of $64\times64$ for MobileNetV2~\cite{sandler2018mobilenetv2} and ProxylessNAS~\cite{cai2019proxylessnas}, and $96\times96$ for MnasNet~\cite{tan2019mnasnet}. The width multipliers are 0.35 for MobileNetV2, 0.3 for ProxylessNAS and 0.2 for MnasNet. 

\section{Design Cost}

There are billions of IoT devices with drastically different constraints, which requires different search spaces and model specialization. Therefore, keeping a low design cost is important. 

MCUNet is efficient in terms of neural architecture design cost. The search space optimization process takes negligible cost since no training or testing is required (it takes around 2 CPU hours to collect all the FLOPs statistics). The process needs to be done only once and can be reused for different constraints (\eg, we covered two MCU devices and 4 memory constraints in Table 4). TinyNAS is an one-shot neural architecture search method without a meta controller, which is far more efficient compared to traditional neural architecture search method: it takes 40,000 GPU hours for MnasNet~\cite{tan2019mnasnet} to design a model, while MCUNet only  takes 300 GPU hours, reducing the search cost by 133$\times$. With MCUNet, we reduce the $CO_2$ emission from 11,345 lbs to 85 lbs per model (Figure~\ref{fig:co2_emission}).

\begin{figure*}[h]
    \centering
    \includegraphics[width=0.6\textwidth]{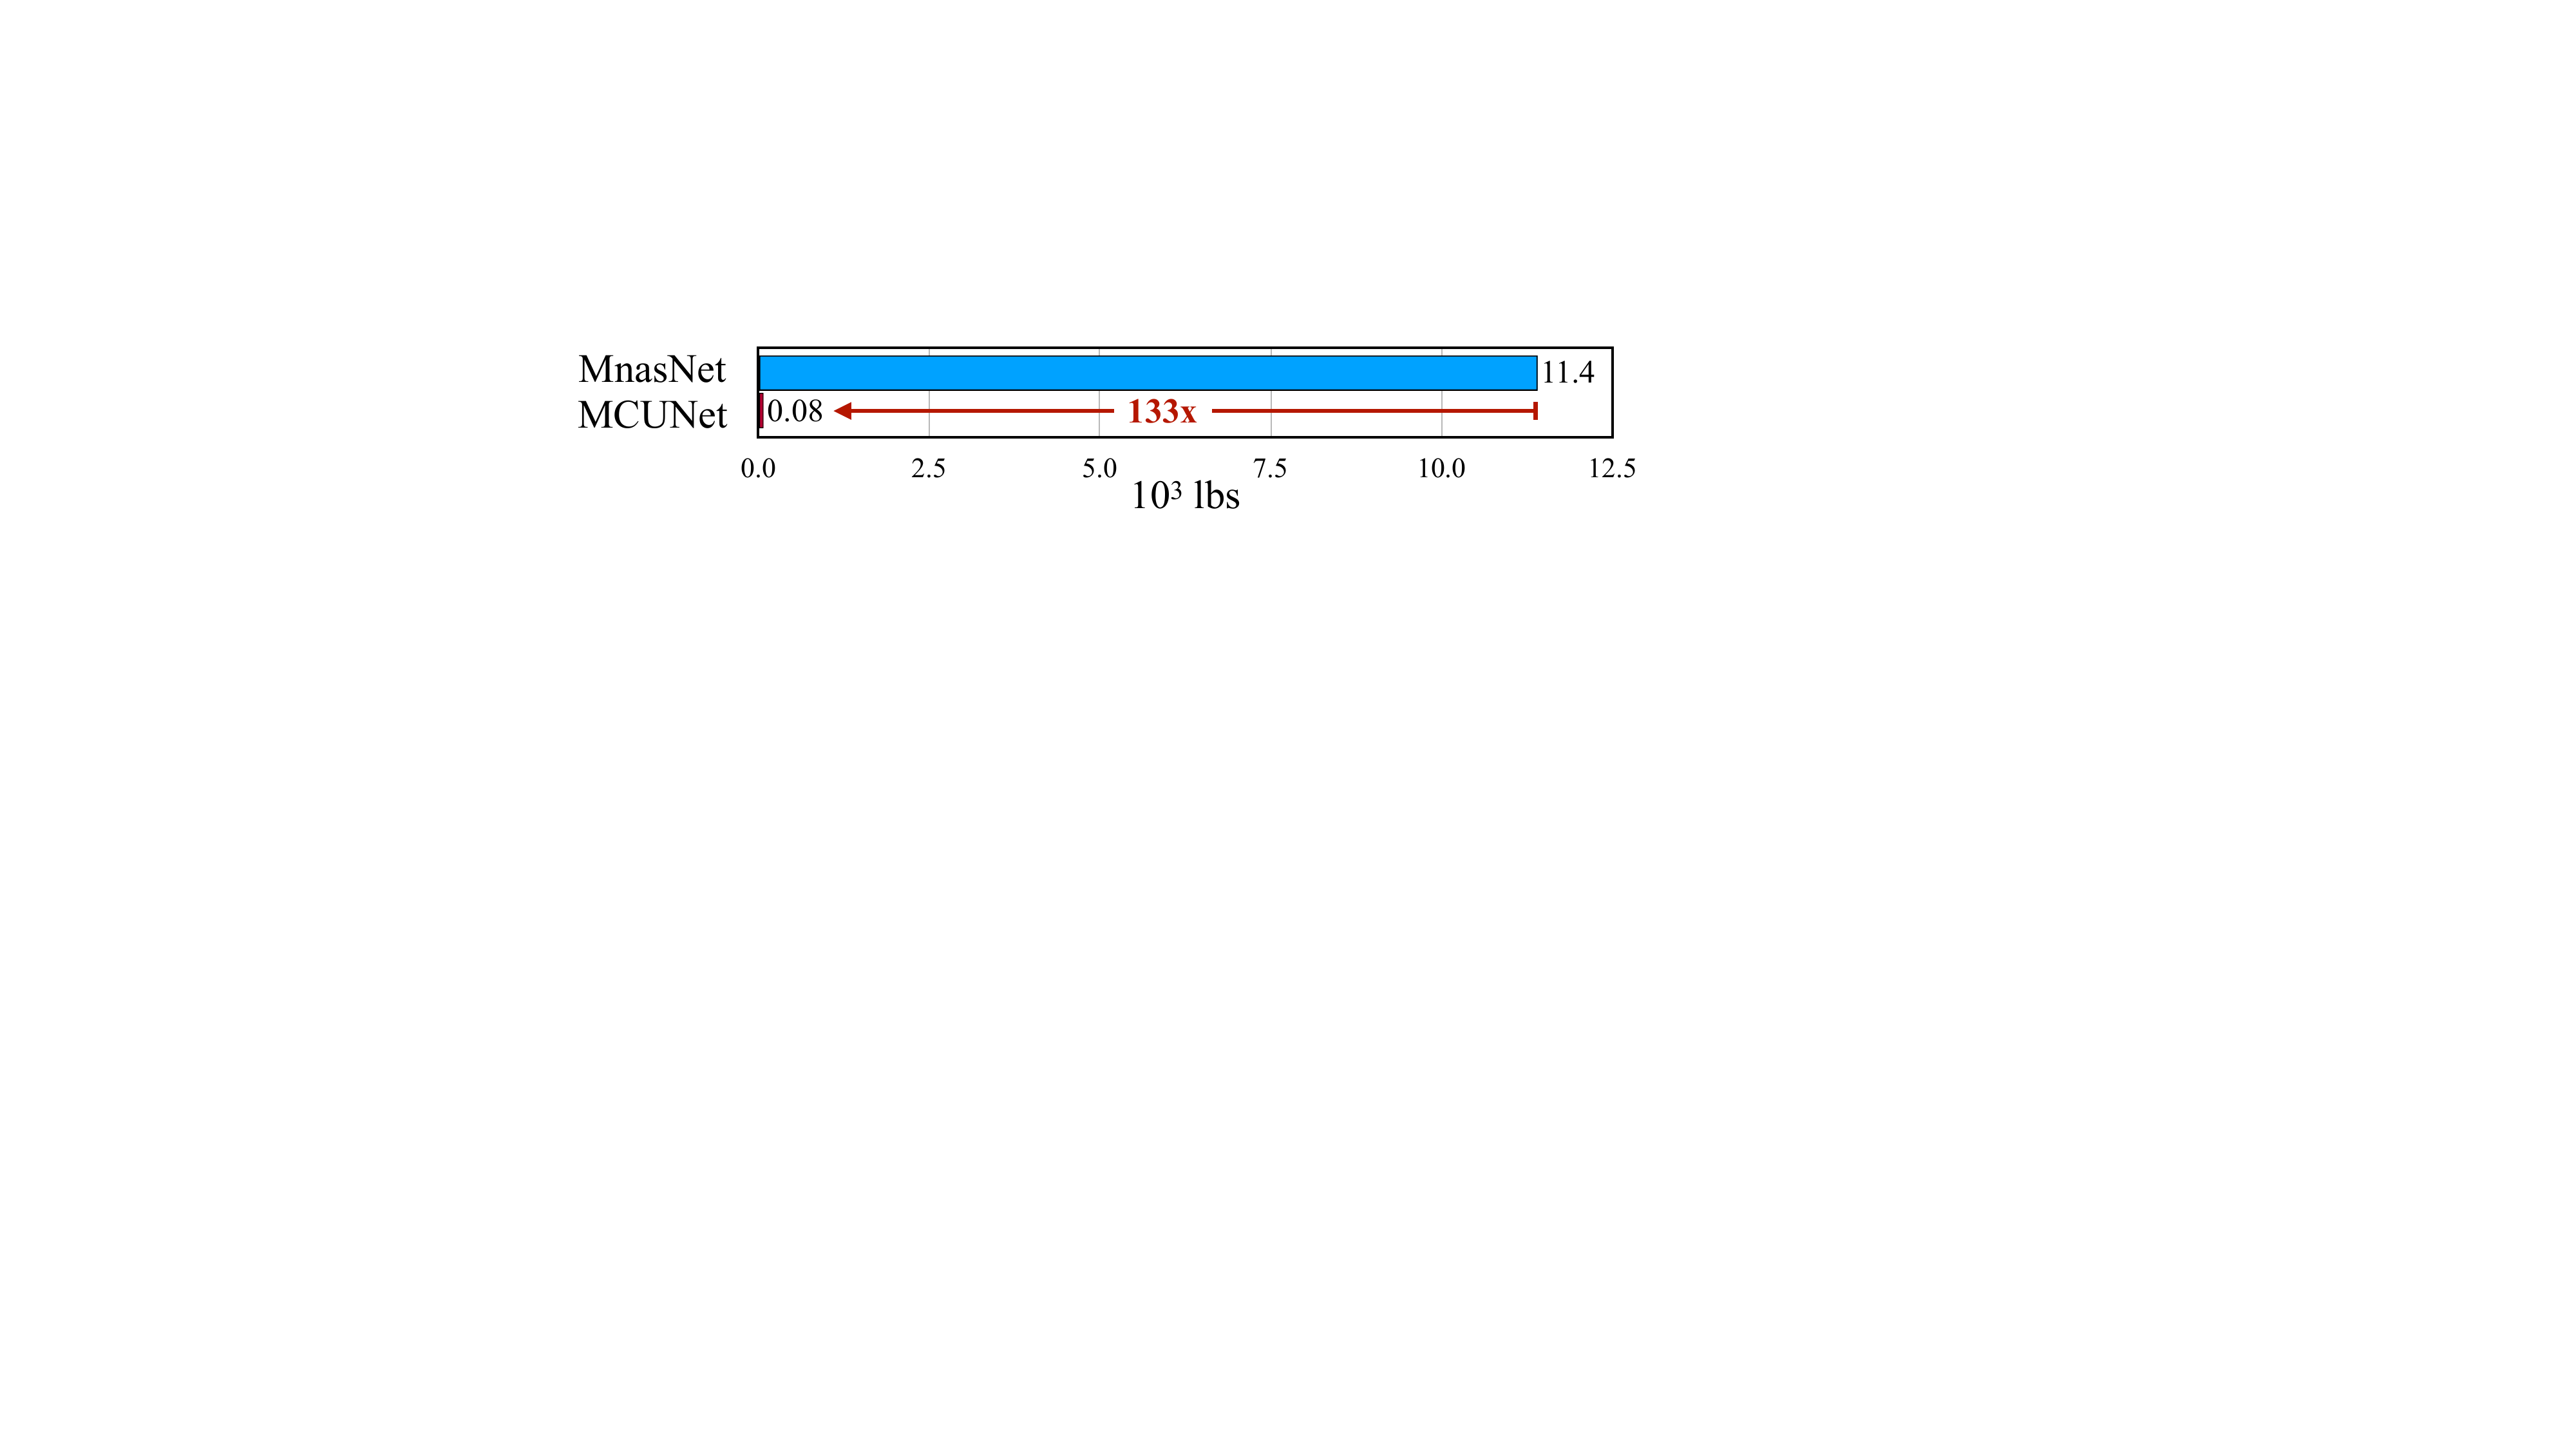}
    \caption{Total $CO_2$ emission (klbs) for model design. MCUNet saves the design cost by orders of magnitude, allowing model specialization for different deployment scenarios.}
    \label{fig:co2_emission}
\end{figure*}

% \SH{design cost: Billions of IoT devices. drastically different constraint. low design cost is important. systematic and automatic design methodology. our framework is portable: (covered two MCU devices and 4 memory constraints in Figure/Table xxx).}

\section{Resource-Constrained Model Specialization Details}

For all the experiments in our paper, we used the same training recipe for neural architecture search to keep a fair comparison.

\myparagraph{Super network training.}

We first train a super network to contain all the sub-networks in the search space through \emph{weight sharing}. Our search space is based on the widely-used mobile search space~\cite{tan2019mnasnet, cai2019proxylessnas, wu2019fbnet, cai2020once} and supports variable kernel sizes for depth-wise convolution (3/5/7), variable expansion ratios for inverted bottleneck (3/4/6) and variable stage depths (2/3/4). The input resolution and width multiplier is chosen from search the space optimization technique proposed in section 3.1. The number of possible sub-networks that TinyNAS can cover in the search space is large: $2\times10^{19}$.

To speed up the convergence, we first train the largest sub-network inside the search space (all kernel size 7, all expansion ratio 6, all stage depth 4). We then use the trained weights to initialize the super network. Following~\cite{cai2020once}, we sort the channels weights according to their importance (we used L-1 norm to measure the importance~\cite{han2015learning}), so that the most important channels are ranked higher. Then we train the super network to support different sub-networks. For each batch of data, we randomly sample 4 sub-networks, calculate the loss, backpropogate the gradients for each sub-network, and update the corresponding weights. For weight sharing, when select a smaller kernel, \eg, kernel size 3, we index the central $3\times3$ window from the $7\times7$ kernel; when selecting a smaller expansion ratio, \eg 3, we index the first $3n$ channels from the $6n$ channels ($n$ is \#block input channels), as the weights are already sorted according to importance; when using a smaller stage depth, \eg 2, we calculate the first 2 blocks inside the stage the skip the rest. 
Since we use a fixed order when sampling sub-networks, we keep the same sampling manner when evaluating their performance.

\myparagraph{Evolution search. }
After super-network training, we use evolution to find the best sub-network architecture. We use a population size of 100. To get the first generation of population, we randomly sample sub-networks and keep 100 satisfying networks that fit the resource constraints. We measure the accuracy of each candidate on the independent validation set split from the training set.
Then, for each iteration, we keep the top-20 candidates in the population with highest accuracy. We use crossover to generate 50 new candidates, and use mutation with probability 0.1 to generate another 50 new candidates, which form a new generation of size 100. We measure the accuracy of each candidate in the new generation. The process is repeated for 30 iterations, and we choose the sub-network with the highest validation accuracy.

\section{Training\&Testing Details}

\myparagraph{Training.} The super network is trained on the training set excluding the split validation set.
We trained the network using the standard SGD optimizer with momentum 0.9 and weight decay 5e-5. 
For super network training, we used cosine annealing learning rate~\cite{loshchilov2016sgdr} with a starting learning rate 0.05 for every 256 samples. The largest sub-network is trained for 150 epochs on ImageNet~\cite{deng2009imagenet}, 100 epochs on Speech Commands~\cite{warden2018speech} and 30 epochs on Visual Wake Words~\cite{chowdhery2019visual} due to different dataset sizes. Then we train the super network for twice training epochs by randomly sampling sub-networks.

\myparagraph{Validation.} We evaluate the performance of each sub-network on the independent validation set split from the training set in order not to over-fit the real validation set.
To evaluate each sub-network's performance during evolution search, we index and inherit the partial weights from the super network. We re-calibrate the batch normalization statistics (moving mean and variance) using 20 batches of data with a batch size 64. To evaluate the final performance on the real validation set, we also fine-tuned the best sub-network for 100 epochs on ImageNet.

\myparagraph{Quantization.} For most of the experiments (except Table 4), we used TensorFlow's int8 quantization (both activation and weights are quantized to int8). We used post-training quantization without fine-tuning which can already achieve negligible accuracy loss. 
We also reported the results of 4-bit integer quantization (weight and activation) on ImageNet (Table 4 of the paper). In this case, we used quantization-aware fine-tuning for 25 epochs to recover the accuracy.

% \section{Accuracy-FLOPs Samples}

% \begin{figure*}[h]
%     \centering
%     \includegraphics[width=0.3\textwidth]{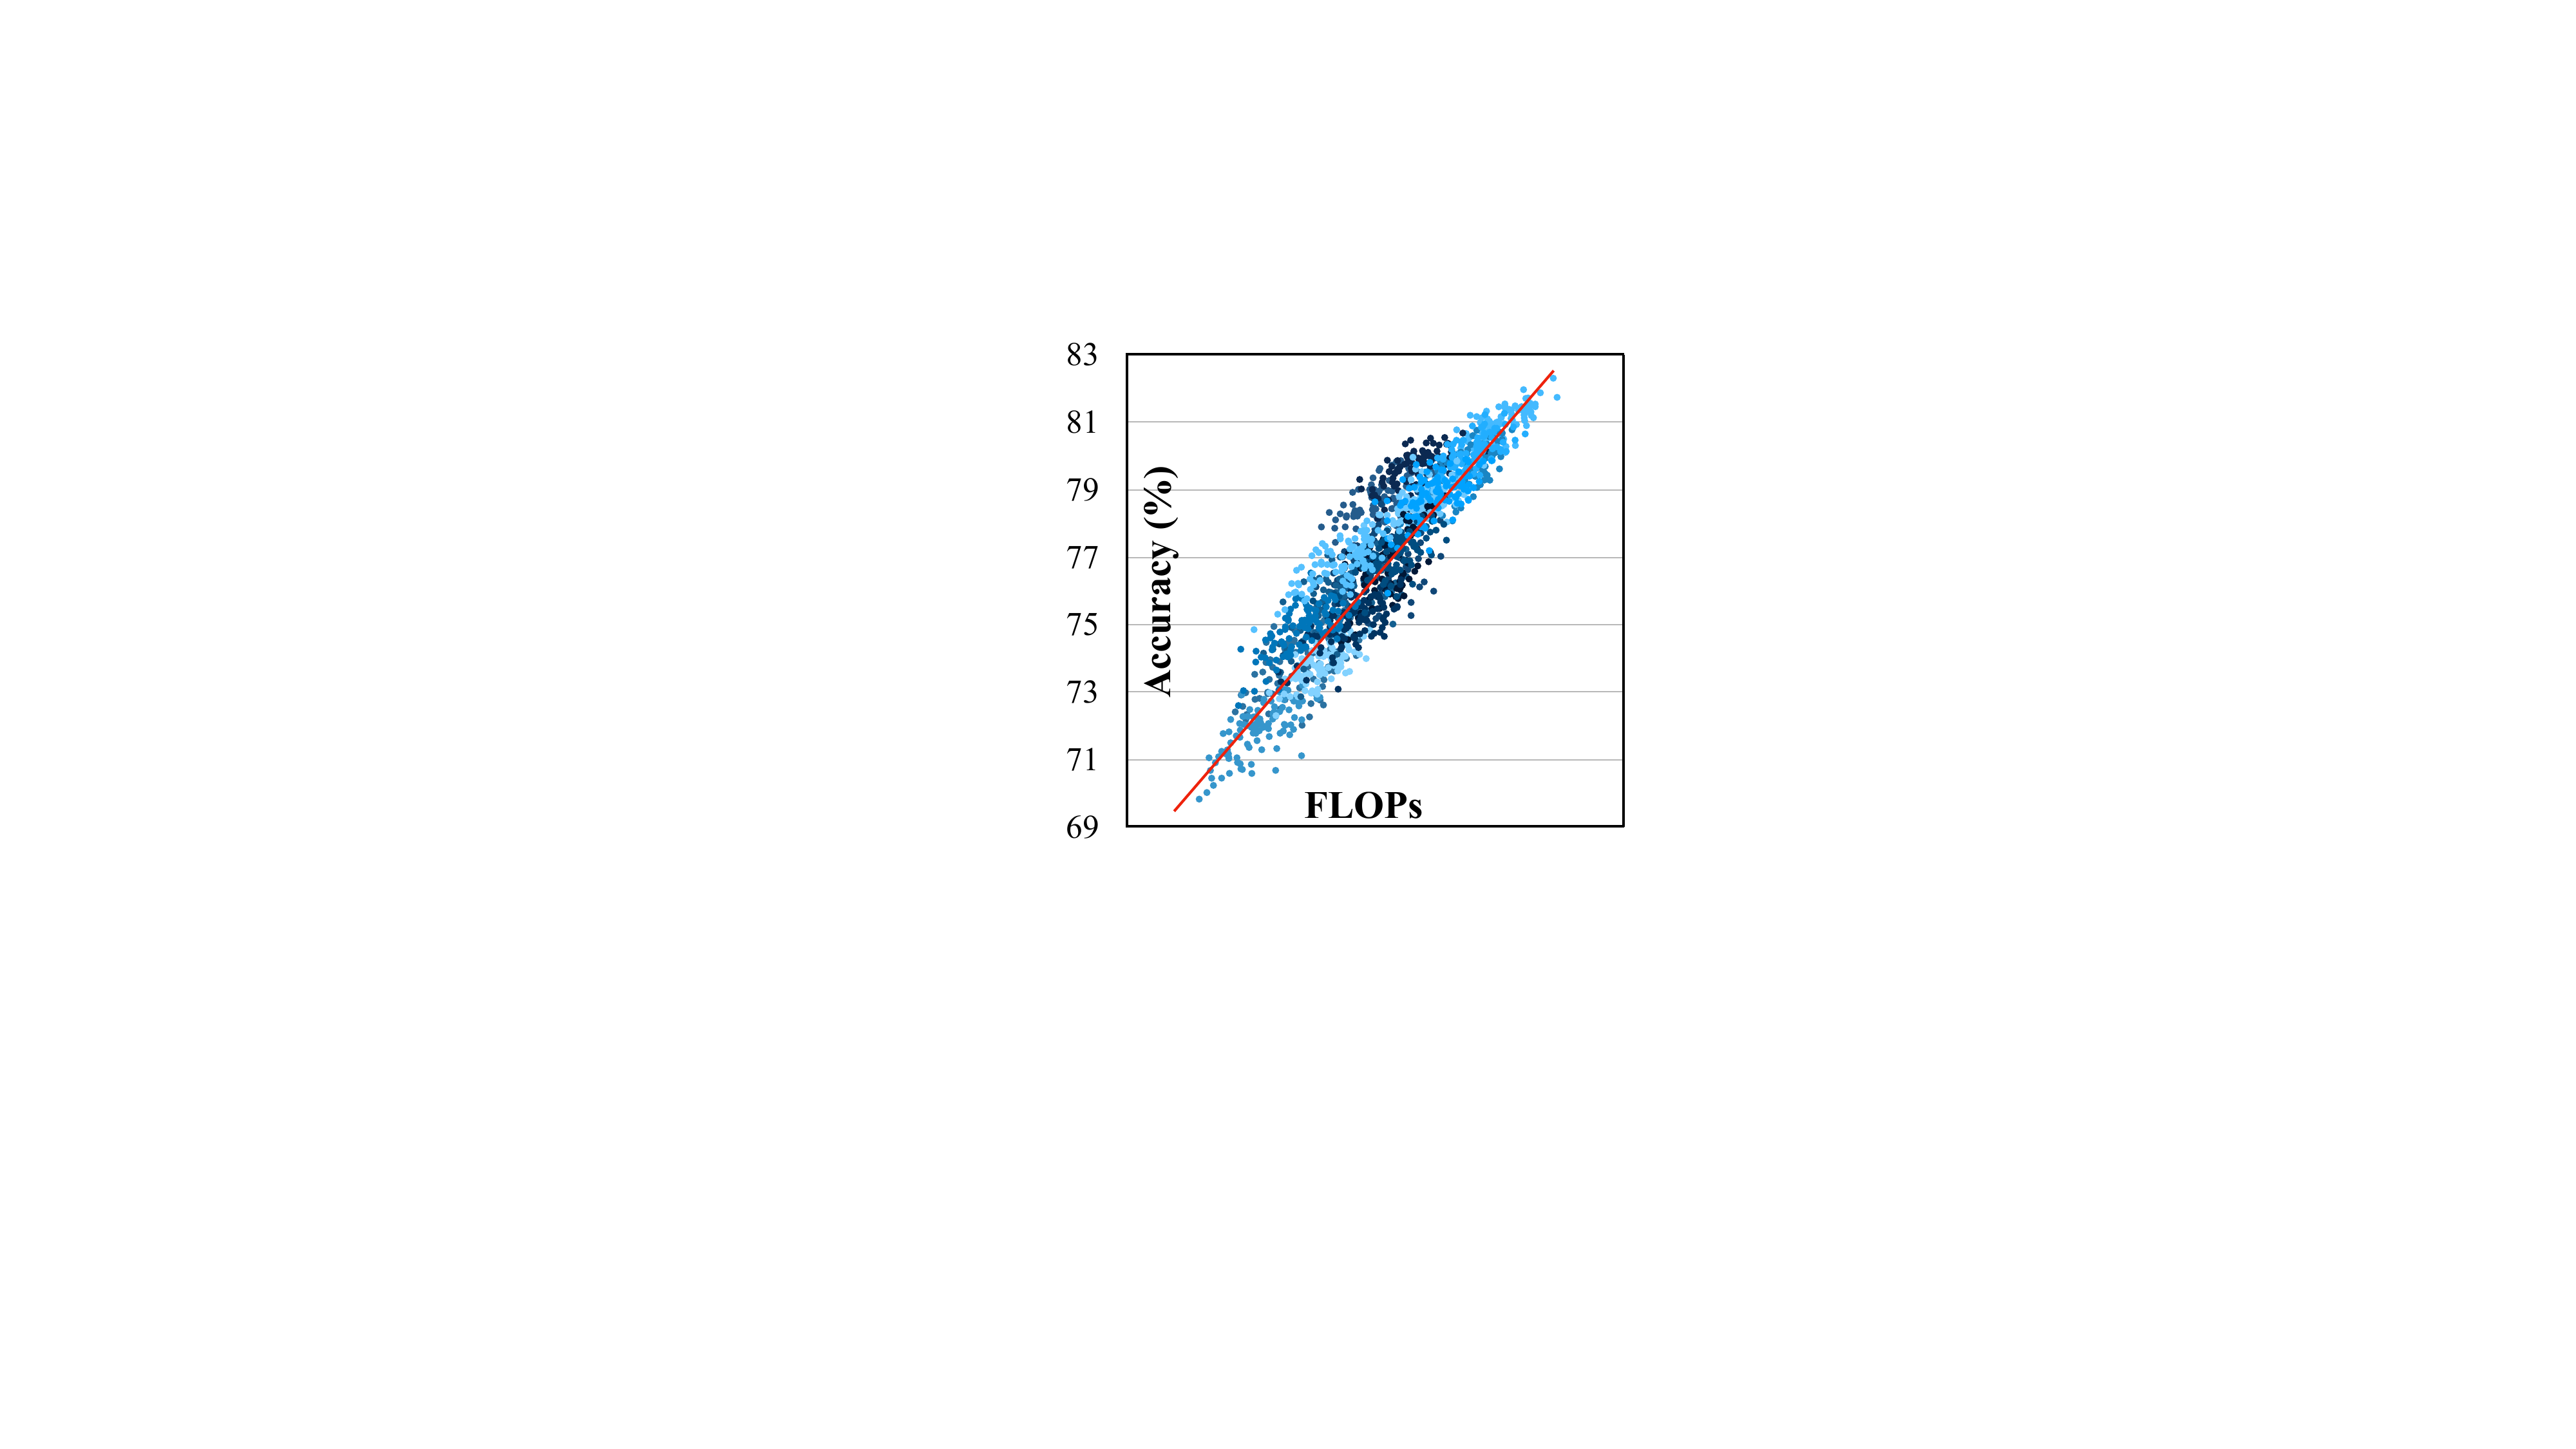}
%     \caption{Distribution of accuracy-FLOPs. We can see a clear positive trend. }
%     \label{fig:acc_flops}
% \end{figure*}

% During automated search space optimization (Section 3.1), we used FLOPs to efficiently measure the priority of different search space configurations. 
% We further analyze the assumption that accuracy is positively related to computation in the same model family on ImageNet-100. We randomly sample 1000 networks from different search spaces and plot the accuracy-computation trade-off. We use the same color for all the points in the same search space. The distribution is shown in Figure~\ref{fig:acc_flops}. We can see a clear positive relationship.

\section{Changelog}

\myparagraph{v1}  Initial preprint release.

\myparagraph{v2}  NeurIPS 2020 camera ready version. We add the in-place depth-wise convolution technique to TinyEngine (Figure~\ref{fig:inplaceDW}), which further reduces the peak memory size for inference. Part of the results in Table~\ref{tab:codesign}, ~\ref{tab:latency_imagenet}, ~\ref{tab:4bit} are updated since the new version of TinyEngine can hold a larger model capacity now. The peak SRAM statistics in Figure~\ref{fig:gcommands_curve} are also reduced.
