# Supplementary material for: Tiny Machine Learning: Progress and Futures
Source: arXiv:2403.19076 source file (2024-03-29)
Supplement: Supplementary file 2 [file appendix.tex]

\section{Flow Chart of Contributions}

We provide a flow chart to summarize our contributions in Figure~\ref{fig:supp_flowchart}.
\begin{figure*}[h]
\vspace{-8pt}
    \centering
     \includegraphics[width=1.0\textwidth]{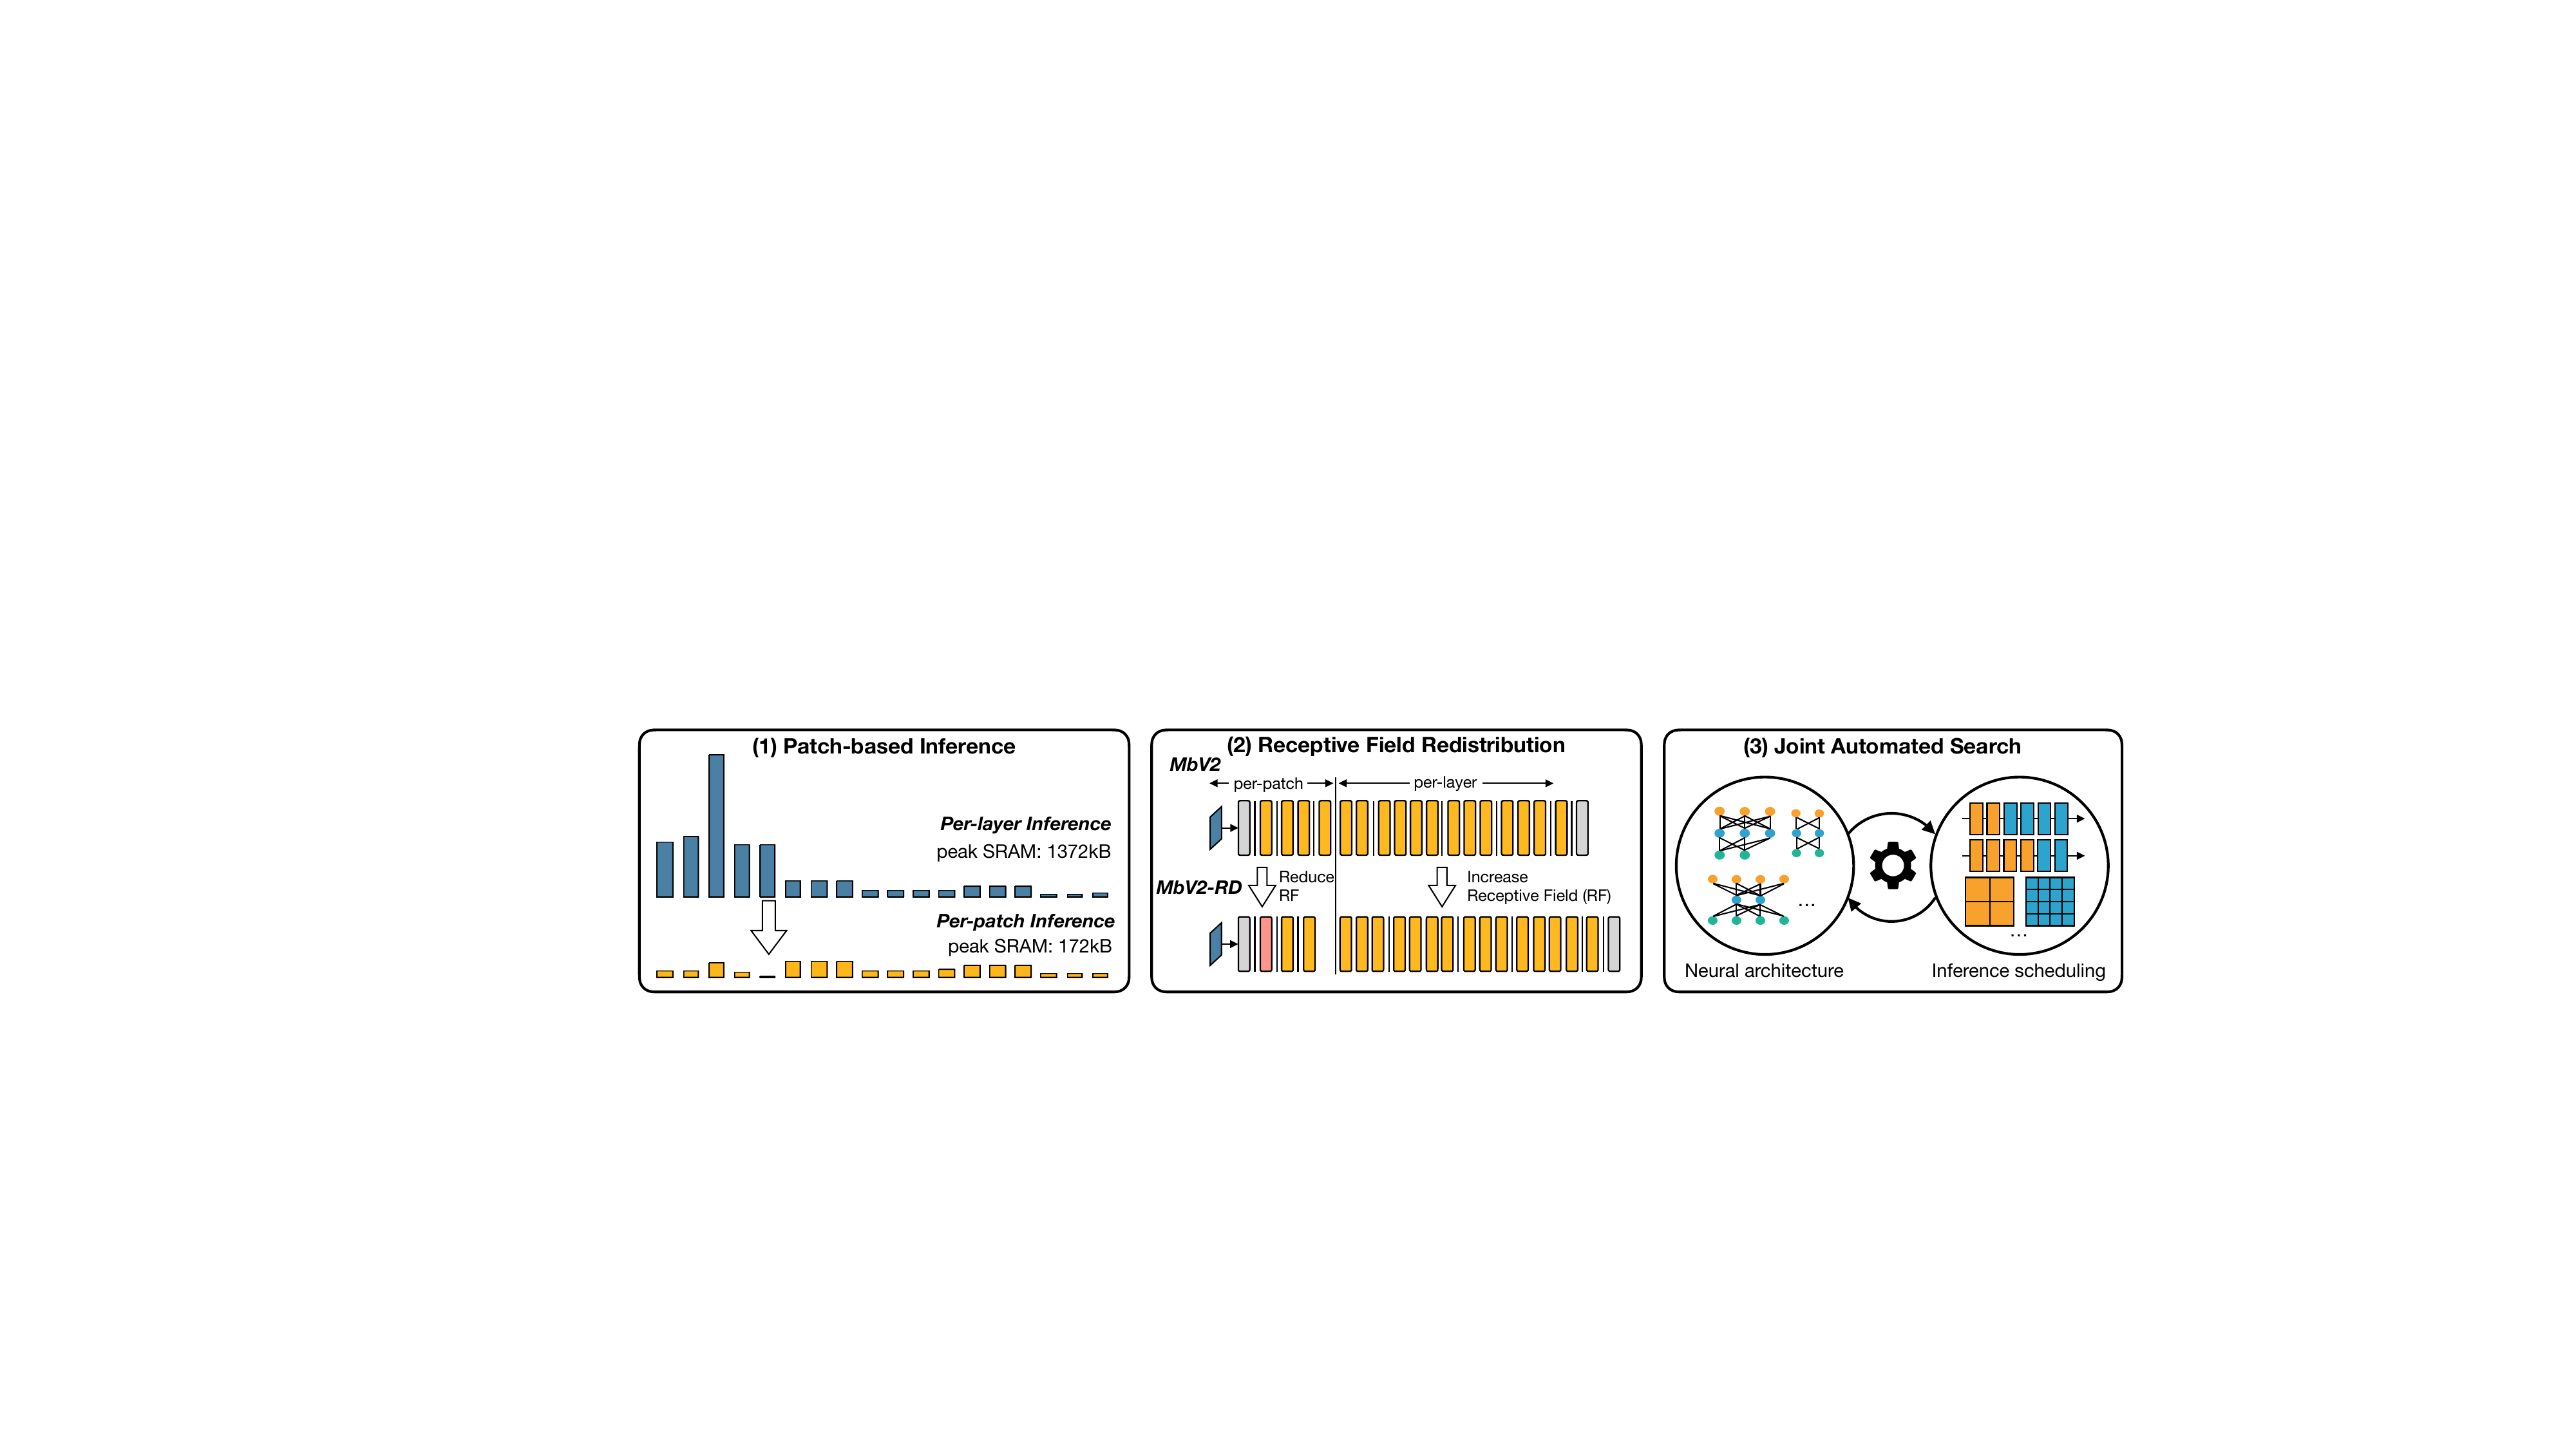}
    \caption{Contributions of \method: (1) Analyze and find the imbalanced memory distribution; propose a patch-based inference scheduling to reduce the peak memory significantly; (2) Propose redistributing receptive fields to reduce the overhead from overlapping patches; (3) Jointly optimize the neural architecture and inference scheduling in the same loop. 
    }
    \label{fig:supp_flowchart}
    \vspace{-10pt}
\end{figure*}

\section{Experimental Details}
\paragraph{Search space.}
We used a MnasNet-alike search space~\cite{tan2019mnasnet, lin2020mcunet, cai2019proxylessnas} for neural architecture search. The search space consists with the following knobs:
\begin{itemize}
    \item Kernel size for each separable convolution block $k_{[~]}$, choosing from $\{3, 5, 7\}$.
    \item Expansion ratio for each inverted residual block $e_{[~]}$, choosing from $\{3, 4, 6\}$.
    \item Number of blocks for each stage $d_{[~]}$, choosing from $\{2, 3, 4\}$.
    \item Width multiplier for each block $w_{[~]}$, choosing from $\{0.5, 0.75, 1.0\}$.
    \item Input image resolution $r$, choosing from $\{96, 128, 160, 192, 224, 256\}$.
\end{itemize}

For the inference scheduling, apart from the optimization knobs inherited from TinyEngine~\cite{lin2020mcunet}, we also include the following knobs:
\begin{itemize}
    \item Number of patches to split the input image $p$, choosing from $\{1, 2, 3, 4\}$ according to the input image resolution. The image will be split into $p\times p$ patches.
    \item Number of layers to run patch-based inference $n, n<N$, where $N$  is the total number of layers. The rest of the network will be run with per-layer inference.
\end{itemize}

\paragraph{Training.}
We follow the training protocol in~\cite{lin2020mcunet} for super network training. The training dataset is randomly split into a sub-training set and validation set. The validation set size is 10,000 for ImageNet~\cite{deng2009imagenet} and 5,000 for other datasets. We first train the largest network in the search space on the sub-training set using SGD with batch size 1024, initial learning rate 0.2, weight decay 4e-5, and a cosine learning rate decay. The training epochs is 150 for ImageNet~\cite{deng2009imagenet} and 30 for VWW~\cite{chowdhery2019visual}.
Afterward, we sort the channels according to their importance (we used L-1 norm for importance estimation~\cite{han2015learning}). 
Then we initialize the super network with the weights and then perform super network training using the same hyper-parameters for twice the epochs. For each iteration, 4 random architectures are sampled, and the gradients are averaged to train the network. 

After getting the sub-network architecture from the evolutionary search, we fine-tuned the networks using 1/10 of the initial learning rate for 10 epochs.

\paragraph{Validation.}
To prevent over-fitting the real validation set, we evaluate the performance of each sub-network on the split validation set. The weights are taken from the super network using indexing. We re-calibrate the batch normalization statistics using 20 batches of data with a batch size 64.

\paragraph{Evolutionary search.}
We used evolutionary search to find the best sub-network architecture under certain constraints. We use a population size of 100. We randomly sample 100 sub-networks satisfying the constraints to form the first generation of population. For each iteration, we only keep the top-20 candidates with the highest accuracy. Then we perform crossover to generate 50 new candidates and mutation to generate another 50, forming a new generation. The mutation rate is 0.1. We repeat the process for 30 iterations and choose the sub-network with the highest accuracy on the split validation set.

\paragraph{Quantization.} We perform int8 quantization following the format in~\cite{jacob2018quantization}. To reduce the accuracy loss from quantization, we perform quantization-aware training for 10 epochs.

\newpage

\section{Memory Distributions of Efficient Models}

We further provide the memory distributions of three efficient models: MnasNet~\cite{tan2019mnasnet}, FBNet~\cite{wu2019fbnet}, and MCUNet-320kB~\cite{lin2020mcunet} in Figure~\ref{fig:supp_mem_distribution}. 
All the models have a highly imbalanced memory distribution, even for MCUNet, which is specialized for memory-constrained settings.
The results demonstrate the generality of the imbalanced memory distribution phenomenon.
Enabling patch-based inference can cut the peak memory usage of the models by 3.5-6.1$\times$. 

\begin{figure*}[h]
    \centering
     \includegraphics[width=1.0\textwidth]{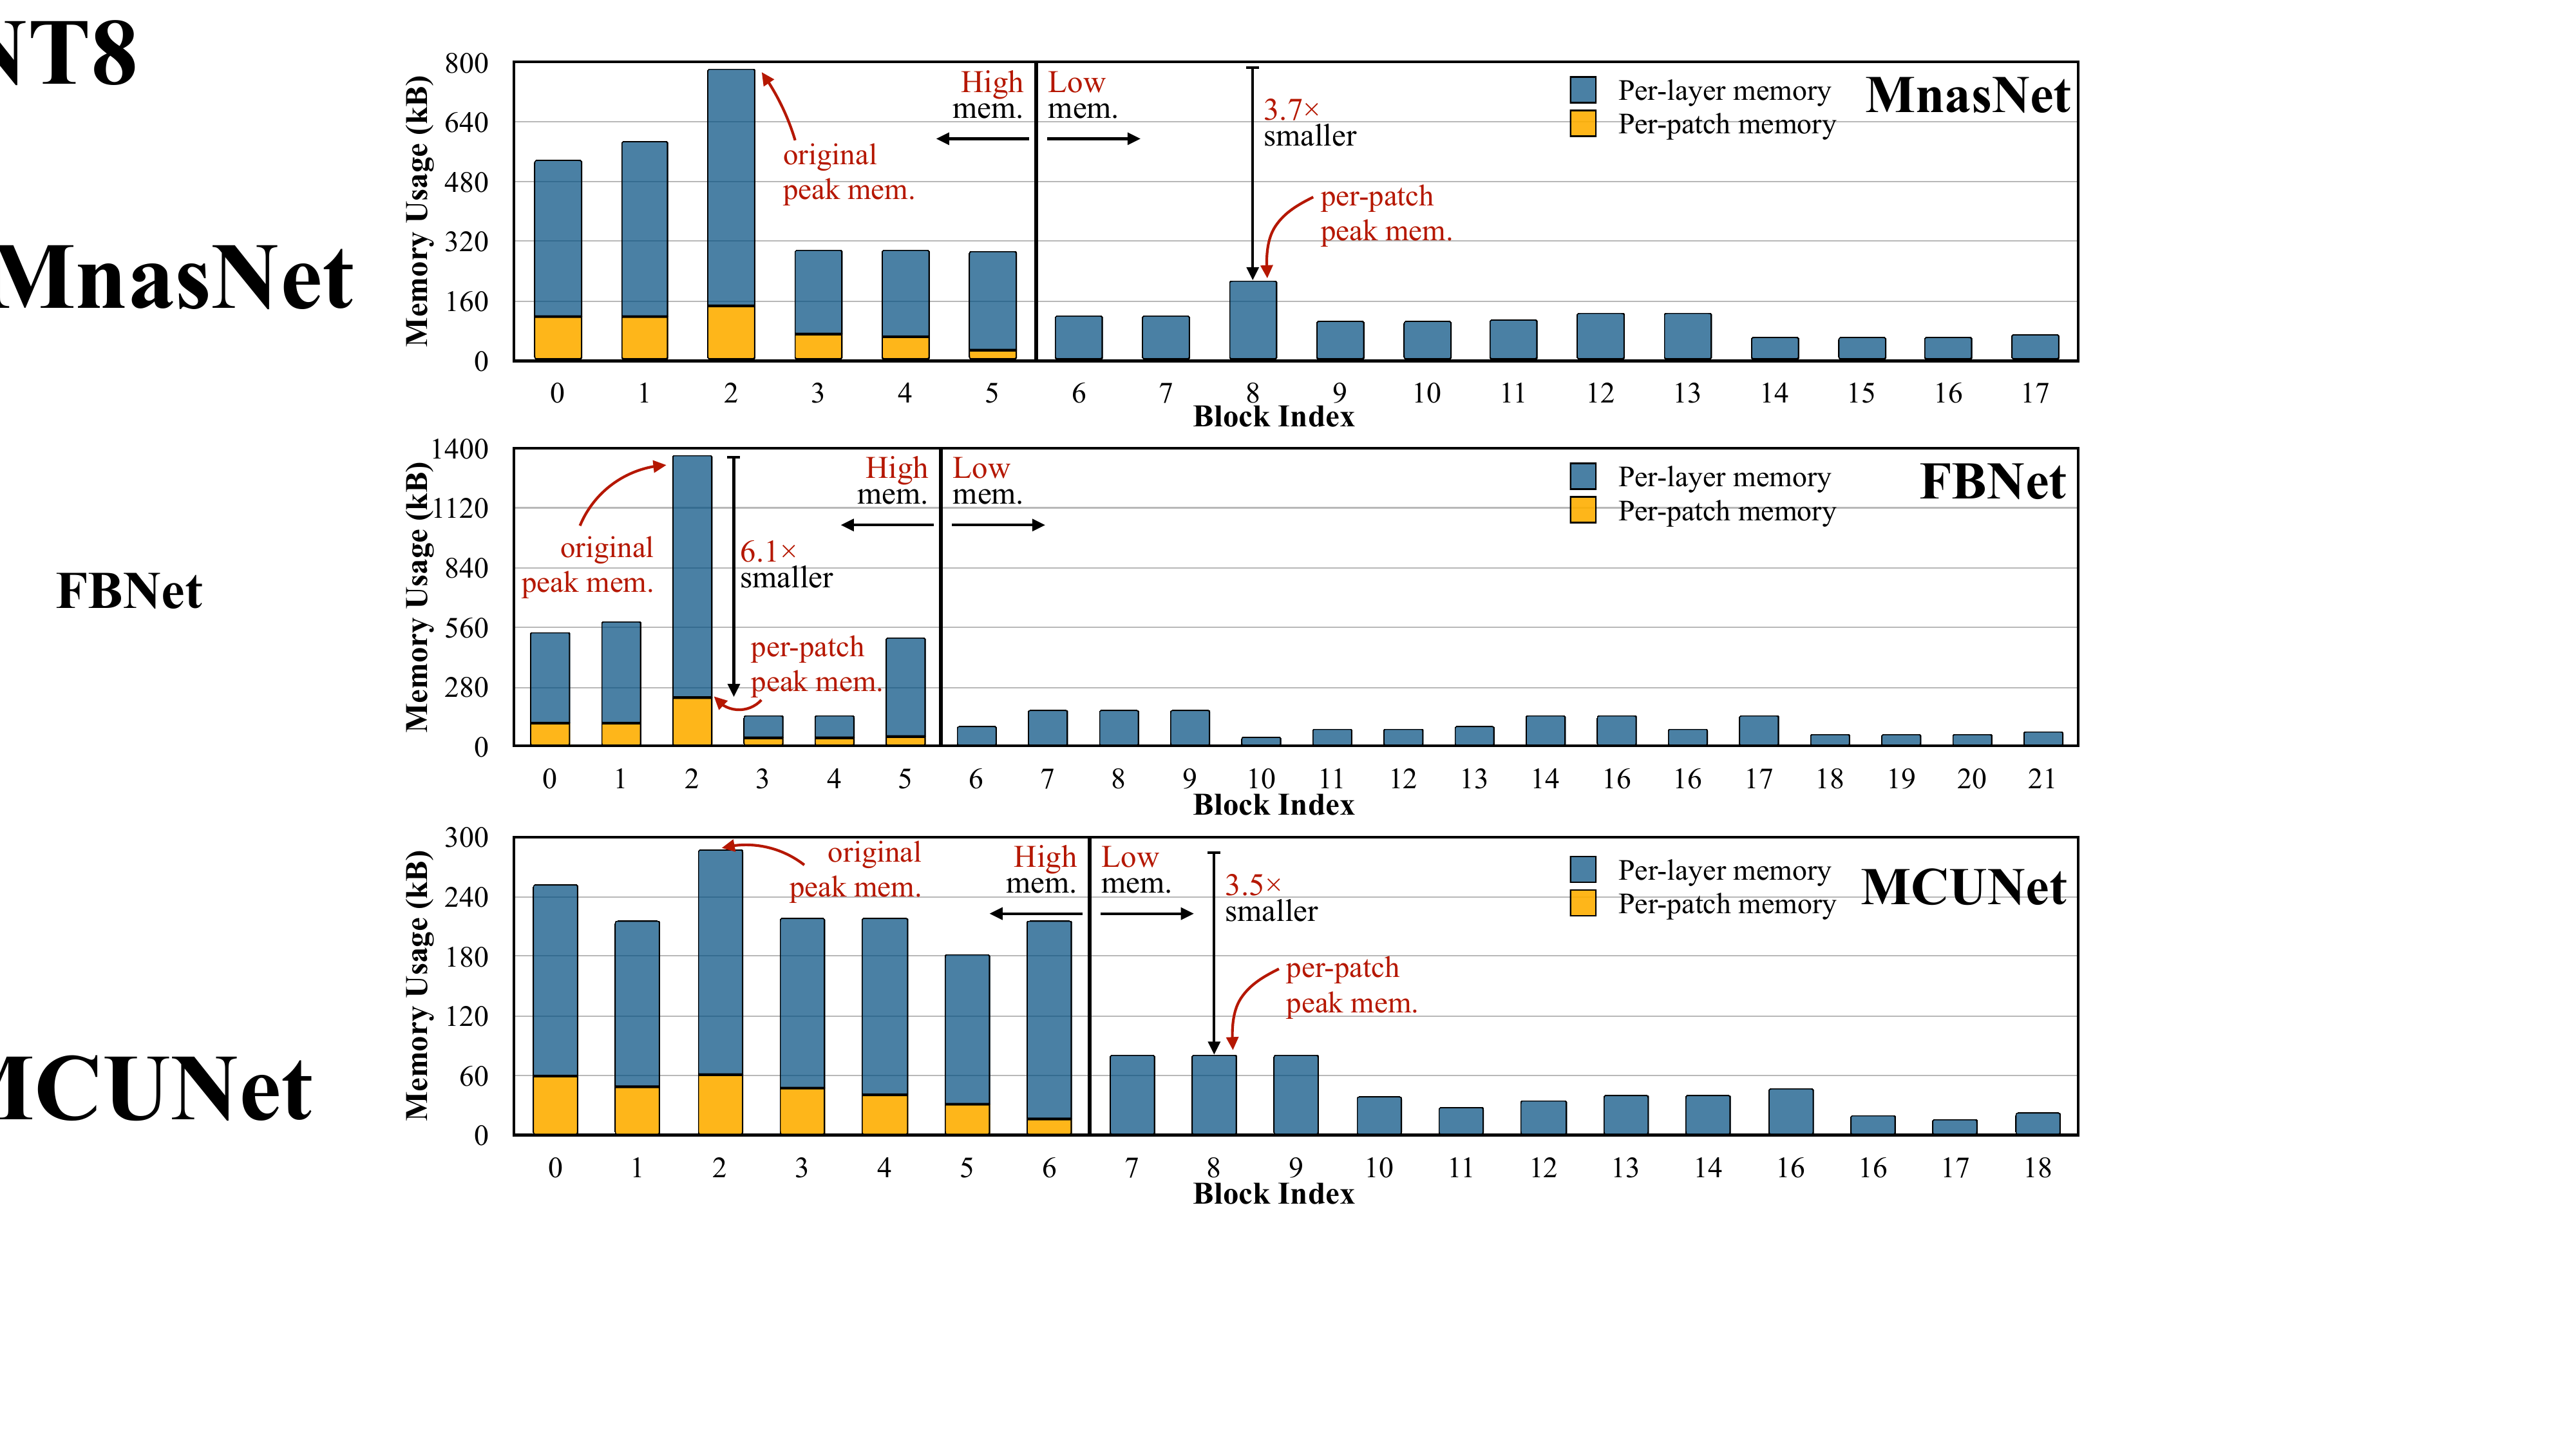}
    \caption{Memory distribution of MnasNet~\cite{tan2019mnasnet}, FBNet~\cite{wu2019fbnet}, and MCUNet-320kB~\cite{lin2020mcunet}.  All the models have an imbalanced memory distribution. Enabling patch-based inference can reduce the peak memory by $3.5-6.1\times$.
    }
    \label{fig:supp_mem_distribution}
\end{figure*}

\newpage

\newpage

\section{Ablation Study on Neural Architecture Search}
Adding width multiplier $w$ and input resolution $r$ in the search space can greatly improve neural architecture search under tiny deep learning settings, because a flexible $r$ and $w$ allows us to globally \emph{scale} the neural network to fit a tight resource budget. This is also mentioned as ``search space optimization'' in~\cite{lin2020mcunet}, where the authors proposed a two-step method that first chooses the optimal $w$ and $r$, and then performs neural architecture search under the given $w$ and $r$. Instead, we merge the two stages by directly adding $r$ and $w$ into the search space.

To show the advantage of our method, we conduct experiments on MobileNetV3~\cite{howard2019searching} space by extending it to support different $r$'s and $w$'s. We compared it with state-of-the-art methods under different computation budgets in Table~\ref{tab:compare_nas}.
Our NAS method consistently outperforms existing techniques for tiny networks in terms of computation-accuracy trade-off. Existing techniques usually need a scaling method to scale down the searched network and fit different budgets. With the extended search space, all our models are derived from the \emph{same} super network while obtaining the best accuracy. The accuracy improvement is more significant under a tiny computation setting ($\leq$25M). We also try supporting flexible $w$'s per block, which improves the accuracy for smaller computation budgets. Therefore, we enable flexible $w$'s by default in our experiments.

\begin{table}[h]
    \caption{Our NAS method outperforms existing state-of-the-art tiny networks in terms of computation-accuracy trade-off, especially under tiny computation settings (<50M). All our models are derived from \emph{the same search space}, while obtaining the best accuracy at different budgets.
    For models with \textcolor{red}{*}, we re-measure the MACs and parameters using our profiler.  }
    \label{tab:compare_nas}
    \centering
    \small{
     \begin{tabular}{lllcccc}
    \toprule
  Budget & Model & Setting & MACs & Weights & Top-1  & Top-5 \\  
  \midrule
\multirow{2}{*}{\shortstack{100M\\MACs}} & MobileNetV1 0.5$\times$ (r=192)~\cite{howard2017mobilenets} & Manual+Scale & 110M & 1.3M & 61.7\% & 83.6\% \\
& MobileNetV2 0.75$\times$(r=160)~\cite{sandler2018mobilenetv2} & Manual+Scale & 107M & 2.6M & 66.4\% & 87.3\%  \\
& MobileNetV3 Small 1.25$\times$~\cite{howard2019searching} & NAS+Scale & 91M & 3.6M & 70.4\% & - \\
& EfficientNet-B\textsuperscript{-2}~\cite{tan2019efficientnet,han2020model} & NAS+Scale & 98M & 3.0M & 70.5\% & 89.5\% \\
& TinyNet-C~\cite{han2020model}  \textcolor{red}{*} & NAS+Scale & 103M & 2.5M & 71.2\% & 89.7\% \\
 \cmidrule{2-7}
 & Ours (uniform $w$) & Joint Search & 98M & 4.2M & \textbf{72.3\%} & \textbf{90.6\%} \\ 
 & Ours (flexible $w$) & Joint Search & 99M & 3.9M & \textbf{72.3\%} & 90.5\% \\
\midrule
\multirow{2}{*}{\shortstack{50M\\MACs}} & MobileNetV2 0.35$\times$~\cite{sandler2018mobilenetv2} & Manual+Scale & 59M & 1.7M & 60.3\% & 82.9\%\\
 & MnasNet-A1 0.35$\times$~\cite{tan2019mnasnet} & NAS+Scale & 63M & 1.7M & 64.1\% & 85.1\% \\ 
& MnasNet-search1~\cite{tan2019mnasnet} & NAS & 65M & 1.9M &  64.9\% & - \\ 
& EfficientNet-B\textsuperscript{-3}~\cite{tan2019efficientnet,han2020model} & NAS+Scale & 51M & 2.0M & 65.0\% & 85.2\% \\
& TinyNet-D~\cite{han2020model} \textcolor{red}{*} & NAS+Scale & 53M & 2.3M & 67.0\% & 87.1\%\\
& MobileNetV3 Small 1.0$\times$~\cite{howard2019searching} & NAS & 56M & 2.5M & 67.4\% & -\\  %
 \cmidrule{2-7}
 & Ours (uniform $w$) & Joint Search & 50M & 2.8M & 67.9\% & 87.7\% \\
 & Ours (flexible $w$) & Joint Search & 50M & 3.5M & \textbf{68.8\%} & \textbf{88.2\%}\\
\midrule
\multirow{2}{*}{\shortstack{25M\\MACs}} & MobileNetV2 0.35$\times$ (r=160)~\cite{sandler2018mobilenetv2} & Manual+Scale &  30M & 1.7M & 55.7\% & 79.1\% \\
 & MnasNet-A1 0.57$\times$ (r=128)~\cite{tan2019mnasnet} & NAS+Scale & 22M & 1.7M & 54.8\% & 78.1\% \\
 & EfficientNet-B\textsuperscript{-4}~\cite{tan2019efficientnet,han2020model} & NAS+Scale & 24M & 1.3M & 56.7\% & 79.8\% \\ 
 & MobileNetV3 Small 0.5$\times$~\cite{howard2019searching} & NAS+Scale & 23M & 1.6M & 58.0\% & - \\
 & TinyNet-E~\cite{han2020model} \textcolor{red}{*} & NAS+Scale & 25M & 2.0M & 59.9\% & 81.1\% \\ 
  \cmidrule{2-7}
 & Ours (uniform $w$) & Joint Search & 25M & 2.6M & 63.2\% & 84.7\% \\
 & Ours (flexble $w$) & Joint Search & 25M & 3.2M & \textbf{63.9\%} & \textbf{84.9\%} \\ 
    \bottomrule
     \end{tabular}
     }
\end{table}

\newpage

\section{Qualitative Results of Face Detection}

We provide the face detection results on WIDER FACE validation set with RNNPool-Face-Quant~\cite{saha2020rnnpool} and \method{-S}. The quantitative results are shown in Table~\ref{tab:supp_wider_face}, where we follow~\cite{saha2020rnnpool} to calculate the peak memory. Our model has better mAP at 1.3$\times$ smaller peak memory.
The qualitative results are shown in Figure~\ref{fig:supp_vis_widerface}. Our model is more robust to poses and background false positives. 

\def\noparam{1}
\begin{table}[h]
    \setlength{\tabcolsep}{5pt}
    \caption{\method{-S} outperforms RNNPool-Face-Quant~\cite{saha2020rnnpool} on WIDER FACE at 1.3$\times$ smaller peak memory. }
    \label{tab:supp_wider_face}
    \centering
    \small{
     \begin{tabular}{lcccccccccc}
    \toprule
  \multirow{2}{*}{Method}  & \multirow{2}{*}{MACs $\downarrow$} &
  \multirow{2}{*}{Peak Memory $\downarrow$}&  \multicolumn{3}{c}{mAP $\uparrow$} &  \multicolumn{3}{c}{mAP ($\leq$3 faces) $\uparrow$} \\  \cmidrule(lr){4-6}\cmidrule(lr){7-9}
  & & (\texttt{int8}) & Easy & Medium & Hard &  Easy & Medium & Hard \\ \midrule
  RNNPool-Face-Quant~\cite{saha2020rnnpool} & 0.12G & \ifx\noparam\undefined 0.06M & \fi 225kB (1.3$\times$) & 0.80 & 0.78 & 0.53 & 0.84 & 0.83 & 0.81\\
  \method{-S} & \textbf{0.11G} & \ifx\noparam\undefined 0.13M &\fi  \textbf{168kB} (1.0$\times$)  & \textbf{0.85} & \textbf{0.81} & \textbf{0.55} & \textbf{0.90} & \textbf{0.89} & \textbf{0.87}\\
    \bottomrule 
     \end{tabular}
     }
\end{table}

\begin{figure*}[h]
    \centering
    \vspace{-10pt}
     \includegraphics[width=0.95\textwidth]{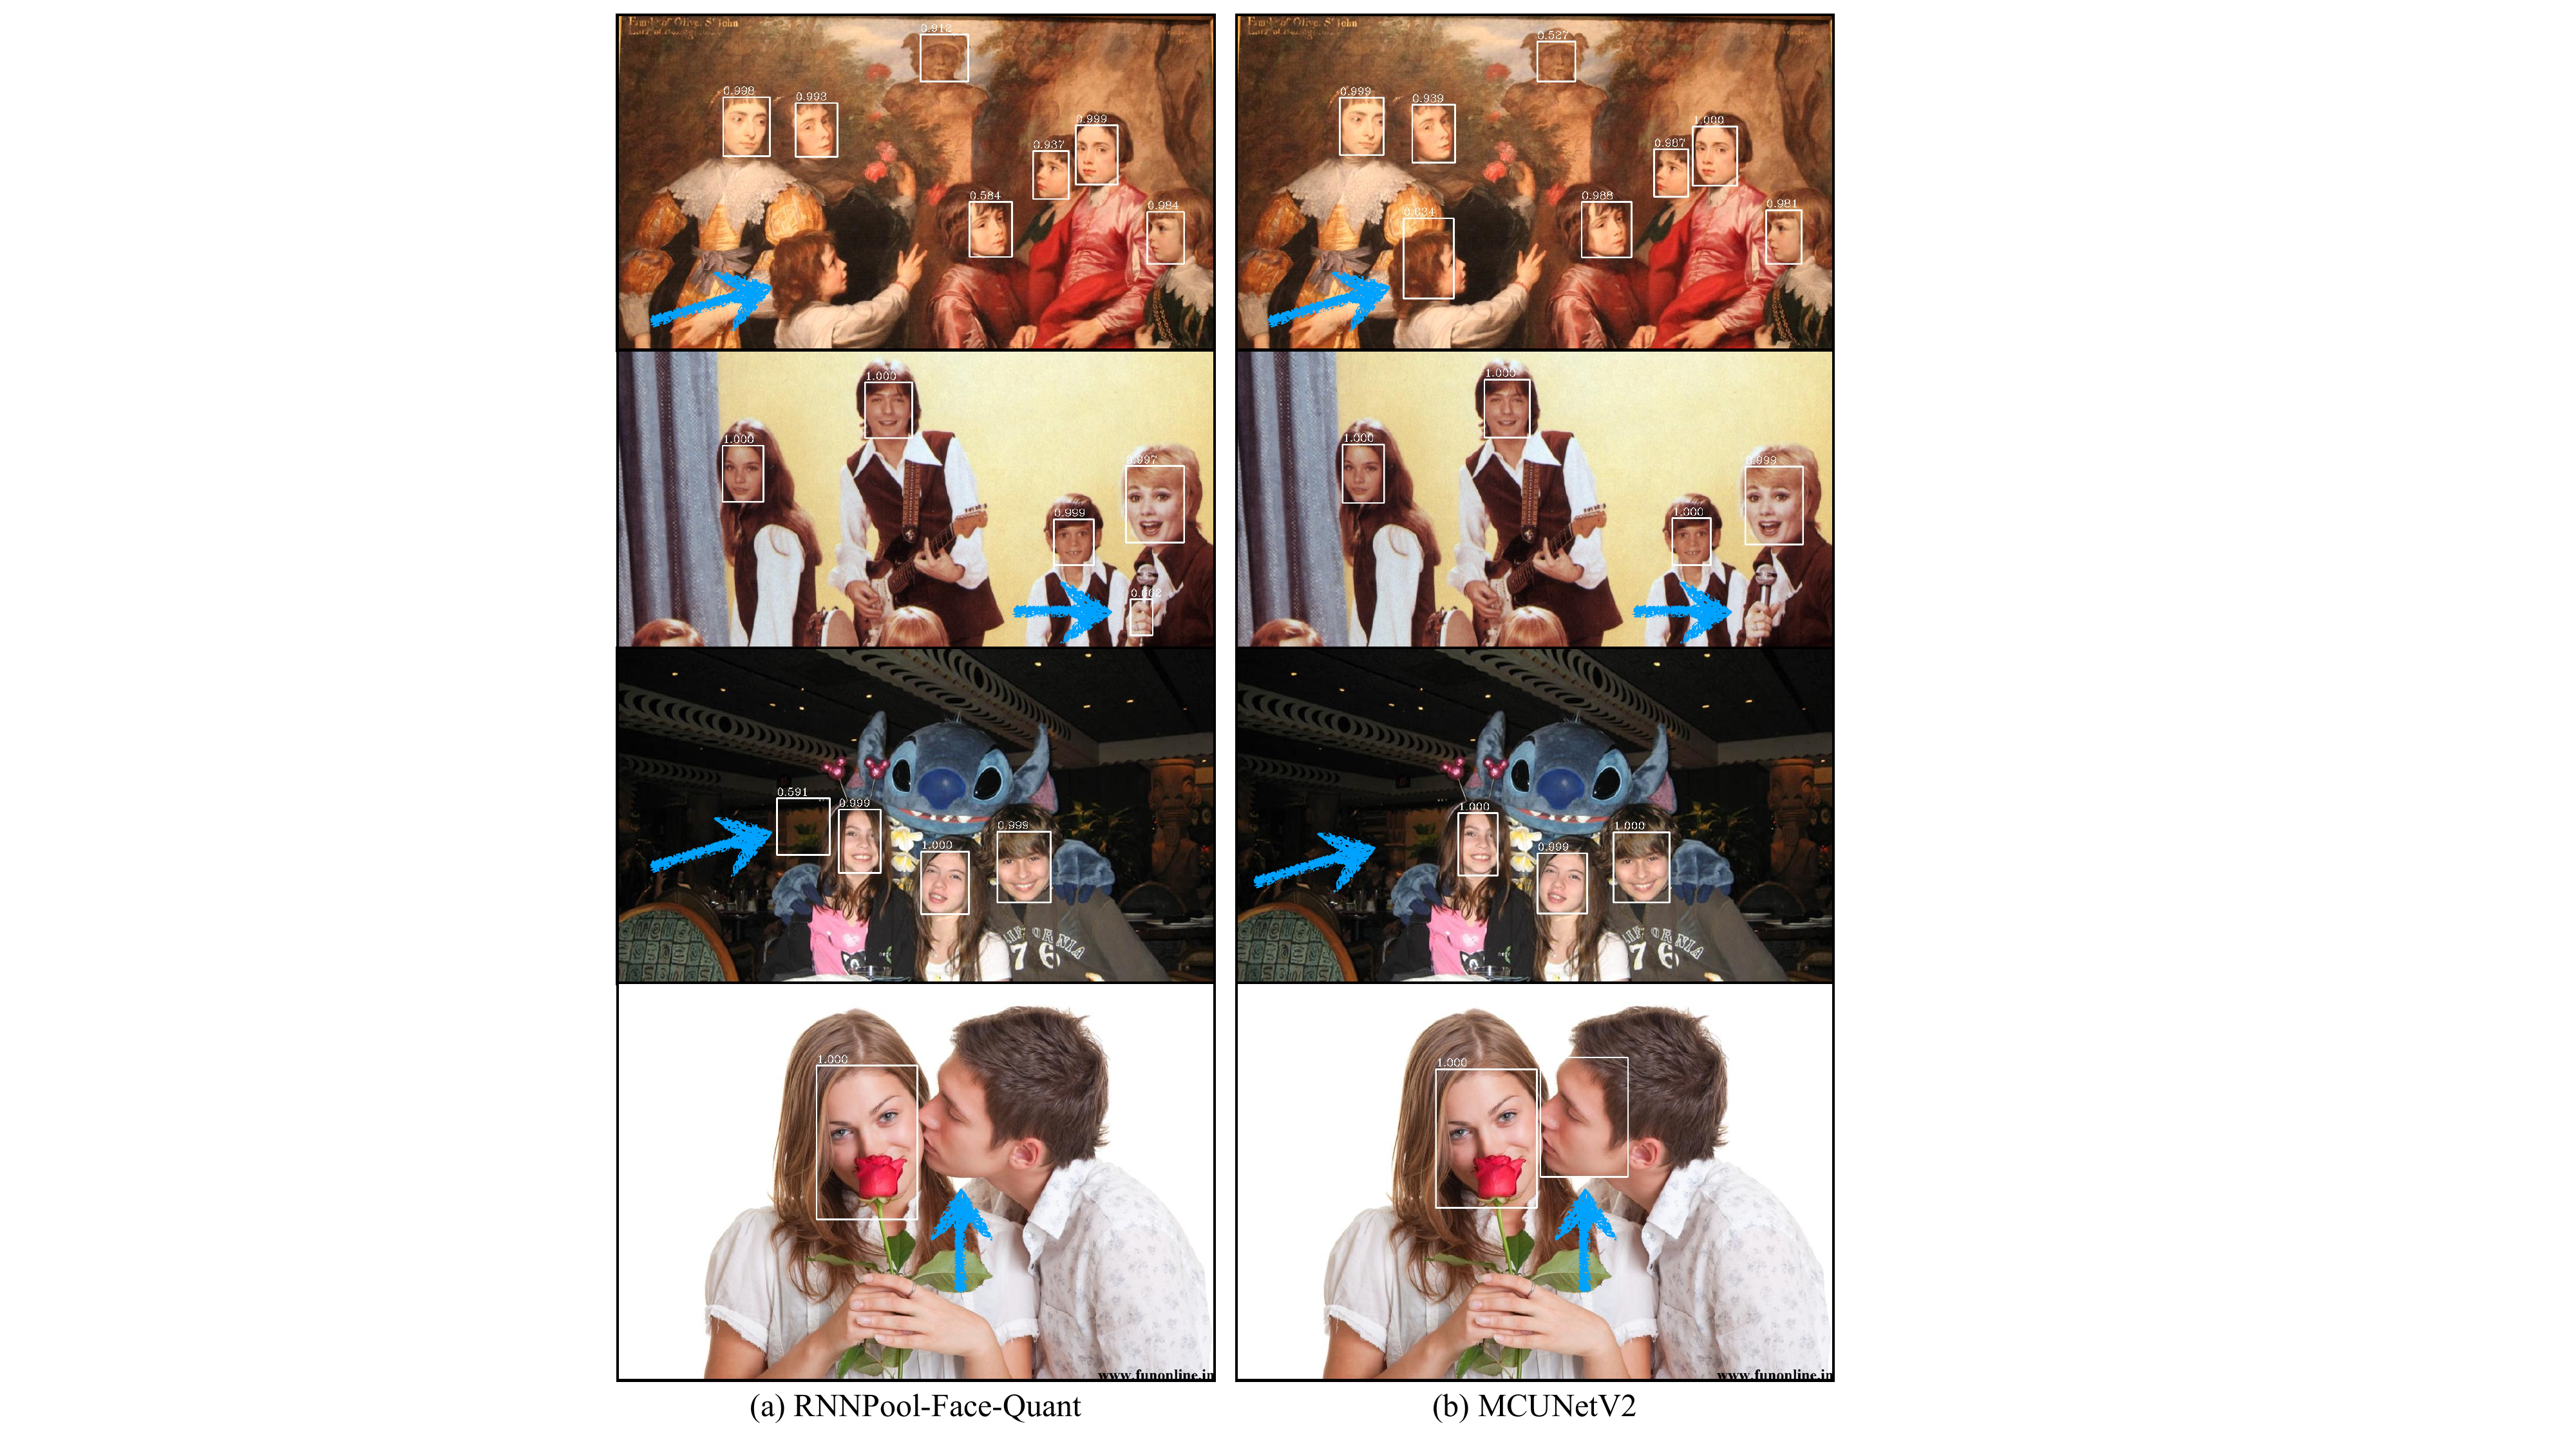}
    \caption{Qualitative results of face detection with RNNPool-Face-Quant~\cite{saha2020rnnpool} and \method{-S} on WIDER FACE~\cite{yang2016wider} validation set. Check the blue arrows: our model is more robust to poses and background false positives. The predictions are filtered with confidence threshold $0.5$.
    }
    \label{fig:supp_vis_widerface}
\end{figure*}

\newpage

\newpage
